# Supplementary material for: Reconstructing Spatiotemporal Data with C-VAEs
Source: arXiv:2307.06243 source file (2023-08-28)
Supplement: Supplementary file 1 [file _appendix.tex]

\hl{TODO LIST:}\\
-. Melhorar graficos (ok por agora)\\
-. Estudo poligonos para enumeracao pros e cons algoritmos \\
-. Continuar a detalhar Metodologia e Interpretacao Resultados - \\
-. Introducao e conclusão
- Notacao math ou normal? 
% \hl{NOTAS:}
% Estrutura do trabalho:
% 1-Introducao; 
% 2-Background and Related Work - no background não se fala dos VAE; Se apresenta os outros métodos.
% 3-Simulation of Polygon Evolution (3.1 - VAE - VAE-based Interpolation; 3.2 - Compression methods (?); 3.3 - Temporal Consistency Metrics); 
% 4 - Performance Evaluation (4.1- Dataset; 4.2 - Results; 4.3 - Discussion); 
% 5 - Conclusion 

https://ieeexplore.ieee.org/document/1348341
Spatiotemporal Databases

\hl{\\Topicos introducao}

0.1. Representação contínua providencia potenciais ganhos em termos de gestão de dados (representação comprimida de fenomenos espacio-temporais) [REF]

1. Queremos interpolar polígonos resultantes de segmentação da área ardida.

1.1. breve sumário do trabalho feito na segmentação, inputs e outputs.

\hl{definir "area ardida"}

\hl{geralmente usam Sintetico vs Real}

WKT => imagens => 
Treino pode ser (preprocessamento)

----------- \\

\begin{table}[ht!]
    \fontsize{8pt}{8pt}\selectfont
    \centering
    \caption{\textbf{Distance Based results.} Jaccard Index and Hausdorff Distance metrics for the Shape Based, C-VAE, and Mckenney algorithms using Distance Based sampling on two datasets: U-Net samples and \emph{BurnedAreaUAV} Test Set. The table highlights the mean, standard deviation, and min-max values for both metrics. The best performance for each metric is indicated in bold.}
    \begin{tabular}{@{}lllllclll@{}}
    \toprule
    \multirow{2}{*}{\textsc{Dataset}} & \multirow{2}{*}{\textsc{Algorithm}} & 
    \multicolumn{3}{c}{\textsc{Jaccard Index}} & \multicolumn{1}{c}{\textsc{ }}& \multicolumn{3}{c}{\textsc{Hausdorff Distance}} \\ 
    \cmidrule(l){3-5}
    \cmidrule(l){6-9}
     & &  Mean & SD & min-max & & Mean & SD & min-max \\ 
    \cmidrule(l){0-5}
    \cmidrule(l){6-9}
    \multirow{3}{*}{\begin{tabular}[c]{@{}l@{}}U-Net Samples\end{tabular}}
     & Shape Based & \textbf{0.738} &  \textbf{0.021} & \textbf{0.672-0.788}  & &\textbf{221.245} & \textbf{49.839} & \textbf{66.491-321.025} \\
     & C-VAE & 0.723 & 0.029 & 0.625-0.773 & & 245.071 & 64.773& 99.464-514.118 \\
     & Mckenney & 0.697 & 0.034 & 0.585-0.782 & & 241.100 & 40.852& 106.199-407.791   \\  
    \cmidrule(l){0-5}
    \cmidrule(l){6-9}
    \multirow{3}{*}{\begin{tabular}[c]{@{}l@{}}\textit{BurnedAreaUAV}\\ Test Set\end{tabular}} 
     & Shape Based  & 0.910 & 0.021& 0.887-0.964 & & \textbf{60.815} &  \textbf{33.312} & \textbf{19.444-117.000}\\
     & C-VAE & \textbf{0.930} & \textbf{0.011} & \textbf{0.889-0.928} &  &85.220 & 14.827 & 52.773-108.853  \\
     & Mckenney & 0.850 & 0.038 & 0.799-0.960 & & 103.068  & 30.744 & 23.014-146.521  \\ 
     \bottomrule
    \end{tabular}
\end{table}

\begin{table}[ht!]
%\fontsize{10pt}{10pt}\selectfont
\centering
\caption{\textbf{Distance Based Sampling Temporal Consistency.} Results of average of the strides of the Temporal Consistency for C-VAE, Shape Based, and Mckenney algorithms, using distance based sampling. Mean, standard deviation (SD), and min-max values are reported. The best performance for each metric is highlighted in bold.}
\begin{tabular}{@{}llll@{}}
\toprule
\multirow{2}{*}{\textsc{Algorithm}} & \multicolumn{3}{c}{\textsc{Avg. Temp. Consistency}} \\
\cmidrule(l){2-4}
& Mean & SD & min-max\\
\midrule
Shape Based & 0.994 & 0.006 & 0.985-1.000 \\
C-VAE & \textbf{0.999} & \textbf{0.001} & \textbf{0.997-1.000} \\
Mckenney & 0.983 & 0.018 & 0.948-0.998 \\
\bottomrule
\end{tabular}
\label{tab:distance_tc}
\end{table}

\begin{figure}[h] 
     \centering
        \centering
        \subfloat{
            \includegraphics[width=0.495\textwidth]
            {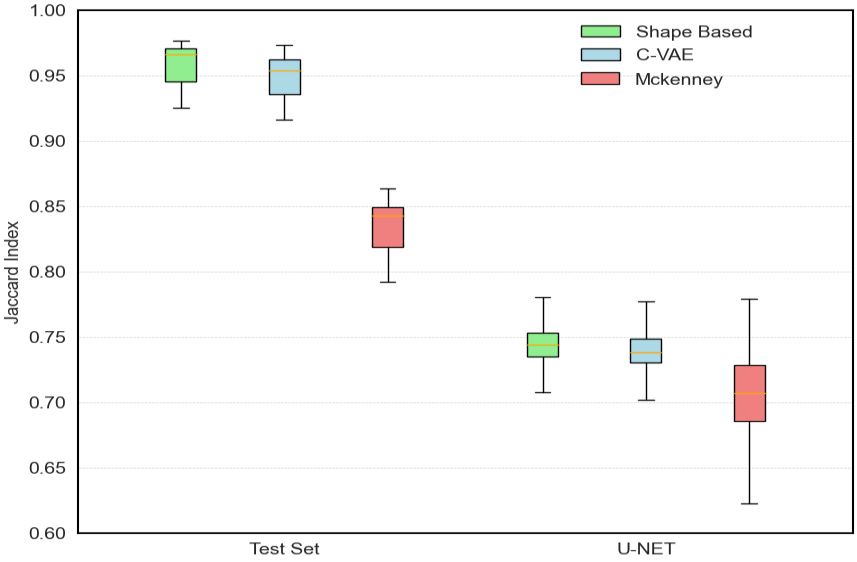}}
     \hfill
         \subfloat{\includegraphics[width=0.495\textwidth]
         {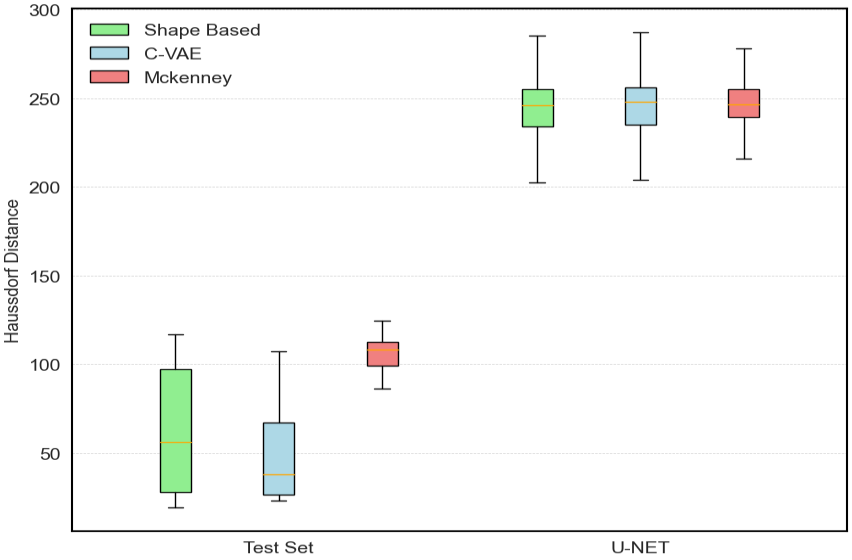}}
         \subfloat{
            \includegraphics[width=0.495\textwidth]
            {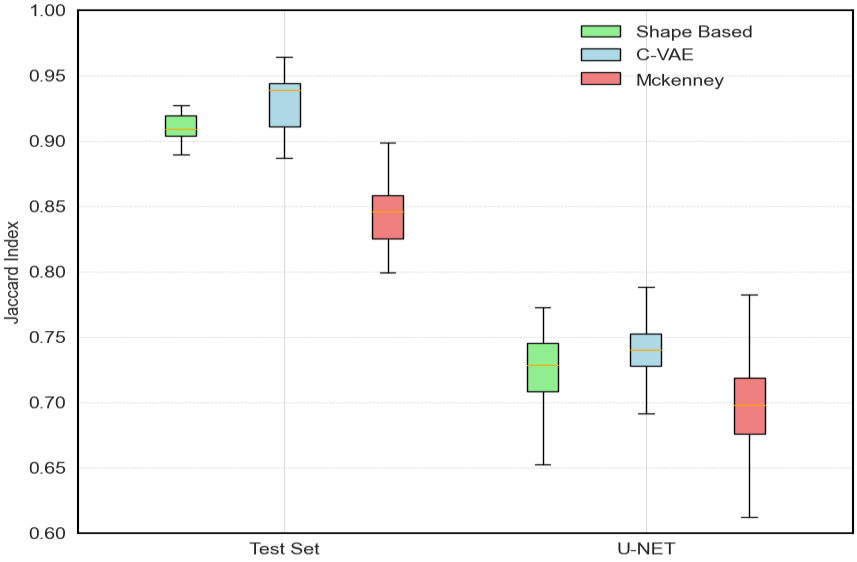}}
     \hfill
         \subfloat{\includegraphics[width=0.495\textwidth]
         {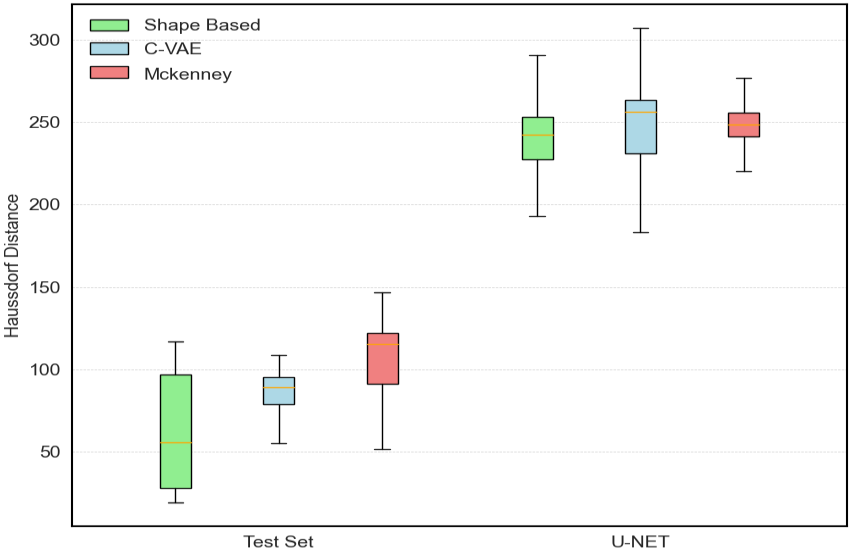}}    
     \caption{\textbf{Periodic Sampling.} caption.}
     \label{fig:iou_hd_periodic}
\end{figure}

\begin{figure}[ht!] 
     \centering
        \centering
        \subfloat{
            \includegraphics[width=0.495\textwidth]
            {imgs/IoU_sampled.png}}
     \hfill
         \subfloat{\includegraphics[width=0.495\textwidth]
         {imgs/HD_sampled.png}}
     \caption{\textbf{Distance Sampling.} caption.}
     \label{fig:iou_hd_sampled}
\end{figure}
